# Supplementary material for: Finding Challenging Metaphors that Confuse Pretrained Language Models
Source: arXiv:2401.16012 source file (2024-01-29)
Supplement: Supplementary file 1 [file appendix.tex]

\section{Number of Metaphors in GLUE}
Statistics of metaphoric sentences in the GLUE benchmark.

\begin{table*}[t]
    \centering
    \resizebox{\textwidth}{!}{
    \begin{tabular}{lcccccccccc}
    \toprule
       & MNLI & QNLI & QQP & RTE & SST & MRPC & STS & WNLI & Avg \\
      \midrule
      \multicolumn{11}{c}{\textbf{\# Metaphors}} 
      \\
      \midrule
    \# Sentence & 20k & 5.4k & 391k & 3k & 1.8k & 1.7k & 1k & 1.4k & 146 & - \\
      \quad At least one & 85\%/17k & 92\%/5k & 74\%/289k & 89\%/2.6k & 92\%/1.6k & 92\%/1.5k & 59\%/.83k & 53\%/10k & 74\% \\
      \quad Critical & 56\%/11.2k & 46\%/2.4k & 27\%/105k & 29\%/0.8k & 48\%/0.9k & 67\%/1.1k & 59\%/.82k & 0\%/0 & 40\% \\
         \bottomrule
    \end{tabular}
    }
    \caption{Number of instances in the GLUE test sets.}
    \label{tab:number_glue}
\end{table*}
